# Supplementary material for: A Study of Finetuning Video Transformers for Multi-view Geometry Tasks
Source: arXiv:2512.18684 source file (2025-12-21)
Supplement: Supplementary file 1 [file optical_flow_AAAI_supp.pdf]

# Supplementary Material for A Study of Finetuning Video Transformers for Multi-view Geometry Tasks

**Huimin Wu**[1], **Kwang-Ting Cheng**[1], **Stephen Lin**[2], **Zhirong Wu**[2]

[1]The Hong Kong University of Science and Technology
[2]Microsoft Research Asia
hwubl@connect.ust.hk, timcheng@ust.hk, stevelin@microsoft.com, wuzhiron@microsoft.com

## Additional Experimental Results

### Visualizing optical flow estimation on KITTI test set.

We also compare with other state-of-the-art approaches on the KITTI test dataset by visualizing flow errors of Image #17 and Image #18. To enhance clarity, we crop the right half and the left half of these two images, respectively. As illustrated in Figure 1, our approach exhibits fewer errors in both background flow prediction (case #1) and foreground flow prediction (case #2).

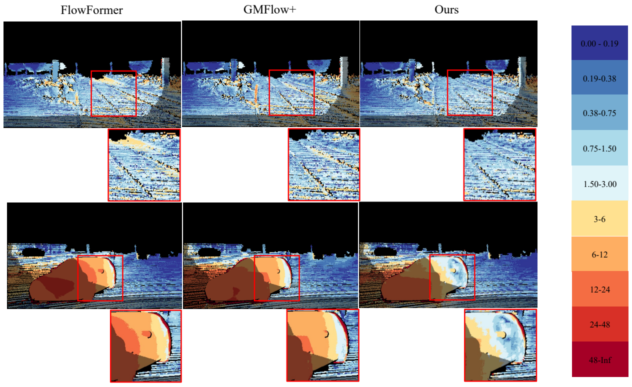


Figure 1: **Visualized comparison on KITTI dataset in terms of prediction error.** The flow error is color-coded the same way as in (Menze and Geiger 2015), with blue indicating correct estimates and red indicating wrong estimates. Our approach is more accurate in both background (case #1) and background (case #2).

### Visualized comparison between simple linear decoding and iterative refinement decoding.

In Figure 2, we demonstrate that the iterative refinement decoding produces superior results on texture-less regions such as road pixels, compared with simple linear decoding.

Copyright © 2026, Association for the Advancement of Artificial Intelligence (www.aaai.org). All rights reserved.

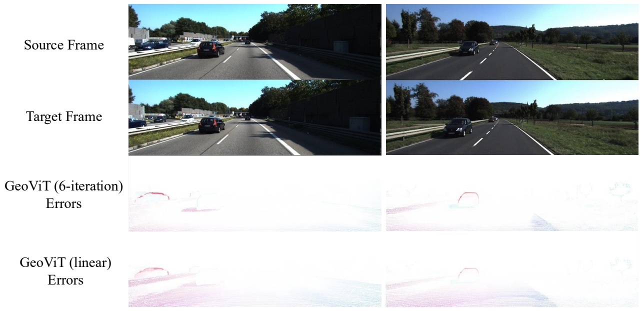


Figure 2: **Visualized comparison on KITTI dataset in terms of prediction error between iterative refinement decoding and linear decoding.** The flow error is color-coded with a darker color indicating larger errors.

| Methods | Inference time (s) | Complexity (M) | Sintel clean | Sintel final |
|---|---|---|---|---|
| Croco v2 (Weinzaepfel et al. 2023) | 19.94 | 437.42 | 1.09 | 2.44 |
| Flowformer++ (Shi et al. 2023) | 2.01 | **16.15** | 1.07 | 1.94 |
| SAMFlow (Zhou et al. 2024) | 1.92 | 22.36 (trainable)<br>659.38 (full) | 0.87 | 2.11 |
| GeoViT (linear) | **0.96** | 303.83 | 0.91 | 2.00 |
| GeoViT (6-iteration) | 5.35 | 375.63 | **0.69** | **1.78** |

Table 1: **Running time comparison with prior arts.** The complexity refers to the number of parameters. GeoViT utilizing iterative refinement decoding achieves the best performance. GeoViT with a linear decoder demonstrates the fastest inference speed with little compromise on performance.

### Running time comparison

We compare the inference time using an NVIDIA GeForce RTX 3090 on the Sintel dataset. We adopt each model's best performing configuration for a system-level comparison. As shown in Table 1, GeoViT with six iterative refinement steps achieves the best results. In terms of running speed, it runs faster than Croco v2 but slower than SAMFlow and Flowformer++. GeoViT with a linear decoder achieves the fastest inference speed without significantly compromising performance.

## References


Menze, M.; and Geiger, A. 2015. Object scene flow for autonomous vehicles. In *Proceedings of the IEEE conference on computer vision and pattern recognition*, 3061–3070.

Shi, X.; Huang, Z.; Li, D.; Zhang, M.; Cheung, K. C.; See, S.; Qin, H.; Dai, J.; and Li, H. 2023. Flowformer++: Masked cost volume autoencoding for pretraining optical flow estimation. In *Proceedings of the IEEE/CVF Conference on Computer Vision and Pattern Recognition*, 1599–1610.

Weinzaepfel, P.; Lucas, T.; Leroy, V.; Cabon, Y.; Arora, V.; Brégier, R.; Csurka, G.; Antsfeld, L.; Chidlovskii, B.; and Revaud, J. 2023. CroCo v2: Improved Cross-view Completion Pre-training for Stereo Matching and Optical Flow. In *Proceedings of the IEEE/CVF International Conference on Computer Vision*, 17969–17980.

Zhou, S.; He, R.; Tan, W.; and Yan, B. 2024. Samflow: Eliminating any fragmentation in optical flow with segment anything model. In *Proceedings of the AAAI Conference on Artificial Intelligence*, volume 38, 7695–7703.
